# Supplementary material for: Learning Versatile Neural Architectures by Propagating Network Codes
Source: arXiv:2103.13253 source file (2022-02-17)
Supplement: Supplementary file 1 [file cls_transfer.tex]

\begin{table*}[t]
  \caption{Single-crop top-1 error rates (\%) of Network Propagation (NP) on the ImageNet validation set.
  The first three models are propagated using neural predictors that are trained on ImageNet-50-1000, ImageNet-50-100, ImageNet-10-1000, respectively.
  The last model is searched by joint optimization of all three predictors.
  $\lambda$ is set to 0.7 during the network propagation process for all searched models.
  FLOPs is measured using an input size of $224\times 224$. Part of this table has been shown in our main paper.
  }
  \centering
%   \footnotesize
  \scalebox{1}{
  \tabcolsep=0.33cm
  \begin{tabular}{l|rr|cc|cc|cc}
    \toprule        
    \multirow{2}{*}{Model} & \multirow{2}{*}{Params} & \multirow{2}{*}{FLOPs} & \multicolumn{2}{c|}{ImNet-50-1000} & \multicolumn{2}{c|}{ImNet-50-100} & \multicolumn{2}{c}{ImNet-10-1000} \\
    & & & top1 & top5 & top1 & top5 & top1 & top5\\
    \midrule
    ResNet$18$~\cite{he2016deep} & 11.20M & 1.82G & 82.72 & 93.88 & 53.04 & 77.64 & 85.00 & 97.40 \\
    ResNet$34$~\cite{he2016deep} & 21.31M & 3.68G & 83.40 & 94.28 & 52.52 & 77.20 & 87.00 & 98.00 \\
    ResNet$50$~\cite{he2016deep} & 23.61M & 4.12G & 83.76 & 94.48 & 50.16 & 75.12 & 86.00 & 98.00\\
    % ResNet$101$~\cite{he2016deep} & 42.60M & 7.85G & 84.32 & 94.80 & 51.92 & 75.72 & 86.00 & 97.80\\
    HRNet-W$18$s~\cite{wang2020deep} & 13.65M & 2.62G & 83.04 & 95.16 & 53.00 & 77.92 & 85.00 & 98.20 \\
    HRNet-W$18$~\cite{wang2020deep} & 19.35M & 4.33G & 83.48 & 94.04 & 50.28 & 76.60 & 83.80 & 98.80 \\
    HRNet-W$32$~\cite{wang2020deep} & 39.29M & 8.99G & 84.00 & 95.12 & 52.00 & 76.48 & 83.80 & 98.40 \\
    % HRNet-W$48$~\cite{wang2020deep} & 75.52M & 17.36G & 84.52 & 94.92 & 52.88 & 77.40 & 86.60 & 98.60 \\
    \midrule
    \textbf{\name-50-1000}~(Fig.~\ref{fig:dynamic-cls-07}) & 4.39M & 5.95G & \textbf{85.80} & 95.36 & 56.04 & 80.20 & 86.80 & 98.20\\
    \textbf{\name-50-100}~(Fig.~\ref{fig:dynamic-cls-50-100-07}) & 3.33M & 3.55G & 82.76 & 94.32 & 56.40 & 81.16 & 85.60 & 99.00\\
    \textbf{\name-10-1000}~(Fig.~\ref{fig:dynamic-cls-10-1000-07}) & 4.06M & 5.51G & 84.60 & 95.12 & 55.60 & 79.92 & 87.80 & \textbf{99.20} \\
    \textbf{\name-All}~(Fig.~\ref{fig:dynamic-cls-abc}) & 4.28M & 6.72G & 85.12 & \textbf{95.56} & \textbf{58.12} & \textbf{82.20} & \textbf{88.20} & 98.20 \\
    \bottomrule
  \end{tabular}
  }
  \label{tab:transfer_cls}
\end{table*}
